# Supplementary material for: Matrix Completion via Residual Spectral Matching
Source: arXiv:2412.10005 source file (2024-12-16)
Supplement: Supplementary file 1 [file Appendix.tex]

\section{Proof sketches for main theorems}
We provide intuitive sketches of technical proofs of key lemmas and theorems presented in Section \ref{sec:theoretical} for ease of readers. Detailed proofs are available in the supplementary material.

Theorem \ref{thm:upper_bound_for_rankr} and its associated corollaries mainly rely on two pivotal Lemmas \ref{lem:loss_for_true} and \ref{lem:large_loss_to_large_error}. The proof of Lemma \ref{lem:loss_for_true} is straightforward. Define that the singular values of $P_{\bOmega}(\bH)/\sqrt{m}\sigma$ as $\theta_1\ge \cdots\ge \theta_n$, the value of loss function can be bounded by
\begin{align*}
        \mathcal{L}(\M_0;\Y,\bOmega) &=
        p^{-1}\sum_{i=1}^n \omega_i \left(\frac{\sigma}{\widehat{\sigma}(\M_0)}\theta_i - \widehat{\lambda}_i\right)^2
        \\&\le 
        p^{-1}\sum_{i=1}^n \omega_i (\theta_i-\widehat{\lambda}_i)^2 + p^{-1}\sum_{i=1}^n \omega_i \left(\frac{\sigma}{\widehat{\sigma}(\M_0)}-1\right)^2\theta_i^2
        \\& \le
        p^{-1} \sup_{1\le i\le n}(\theta_i -\widehat{\lambda}_i)^2 + p^{-1}\theta_1^2 \left(\frac{\sigma}{\widehat{\sigma}(\M_0)}-1\right)^2.
    \end{align*}
Next, we bound the term $\sup_{1\le i\le n}(\theta_i -\widehat{\lambda}_i)$ and $\theta_1$ by establishing the universality for sparse random matrices. The bias $\left|\sigma/\widehat{\sigma}(\M_0)-1\right|$ is controlled though singular value inequalities for low-rank perturbations.

The key argument in proof of Lemma \ref{lem:large_loss_to_large_error} is to demonstrate that when $\|\M-\M_0\|_{F}$ is large, the leading singular values of $P_{\bOmega}(\M-\M_0)$ are likewise large. Consequently, the spectral distribution of $P_{\bOmega}(\bH) + P_{\bOmega}(\M_0 - \M)$ deviates significantly from that of a sparse random matrix, resulting in a substantial increase in the loss function. To formally address this issue, we first demonstrate that a substantial magnitude of $|\bu'(\M-\M_0)\bv|$ for specific directions $\bu\in\mathbb{R}^{m},\bv\in\mathbb{R}^{n}$ with sufficiently small $\|\bu\|_{\infty}$ or $\|\bv\|_{\infty}$ will induce a notable bias in the spectrum of the residual matrix $P_{\bOmega}(\bH) + P_{\bOmega}(\M_0 - \M)$, i.e., 
\begin{align*}
    \|P_{\bOmega}(\bH) + P_{\bOmega}(\M_0 - \M)\| \ge |\bu'P_{\bOmega}(\M - \M_0)\bv| - \|P_{\bOmega}(\bH)\|\gg \|P_{\bOmega}(\bH)\|.
\end{align*}
In this step, the incoherence condition and the constraint of the observation probability $p$ are required. Subsequently, we establish that for any $\M\in \mathbb{M}_{r,\mu_1}$ with a significant error $\|\M-\M_0\|_{F}$, there must exist certain directions, denoted by $\bu\in\mathbb{R}^{m},\bv\in\mathbb{R}^{n}$, which lead to a considerable $|\bu'(\M-\M_0)\bv|$. This is intuitive because when those $|\bu'(\M - \M_0)\bv|$ for different directions $\bu,\bv$ are all small, $\|\M - \M_0\|_F$ is also small, given that the rank of $\M - \M_0$ is low. 

The proof of Theorem \ref{thm:upper_bound_for_convexlambda} appears more complex. Define the singular value decomposition of $\M_0$ and $\widetilde{\M}_{\lambda}$ as $\U\bm{D}\V'$ and $\X \bm{\Theta} \Y'$ respectively, and singular values of $\U'(\M_0 - \widetilde{\M}_{\lambda}) \V$ as $\tau_1\ge\cdots\ge \tau_r$. The nuclear norm of $\widetilde{\M}_{\lambda}$ can be moderately controlled by $\lambda^{-1}\mathcal{L}(\M_0;\Y,\bOmega)$ due to the definition of $\widetilde{\M}_{\lambda}$. Conversely, the lower bound of $\|\widetilde{\M}_{\lambda}\|_{*}$ can be controlled by the singular values $\tau_i$. We partition $\widetilde{\M}_{\lambda}$ into two components: $\M_1 = \operatorname{Proj}_r(\widetilde{\M}_{\lambda})$, representing its projection onto a space of rank $r$, and $\M_2 = \widetilde{\M}_{\lambda} - \M_1$, denoting the residual component. Initially, we constrain $\tau_i$ for $1 \le i \le r$ by acknowledging that a high $\tau_i$ would substantially increase the value of the loss function. This approach mirrors the technique employed in the proof of Lemma \ref{lem:large_loss_to_large_error}. Then, $\|\M_0 - \M_1\|_{F}$ can be controlled when we also similarly investigate the singular values of $\X'_{[1:r]}(\M_0-\widetilde{\M}_{\lambda}) \Y_{[1:r]},\ \X'_{[1:r]}(\M_0-\widetilde{\M}_{\lambda})\V$ and $\U(\M_0-\widetilde{\M}_{\lambda}) \Y_{[1:r]}$. Second, we establish an upper bound for the portion
$(\M_0 - \widetilde{\M}_{\lambda}) - \U\U'(\M_0 - \widetilde{\M}_{\lambda})\V\V'$ by combining the aforementioned bounds for the sum of singular values of $\widetilde{\M}_{\lambda}$ and utilizing the methodology pertaining to relating large singular values to large loss. This help us to derive the bound for $\|\M_2\|_{F}$. Finally, we combine the bounds for $\|\M -\M_1\|_{F}$ and $\|\M_2\|_{F}$ to establish the theorem. 

In section \ref{sec:4.3}, we first establish the properties for the initial value $\M^{(0)}$ in Lemma \ref{lem:bound_for_initial}. The spectral norm error of $p^{-1} P_{\bOmega}(\Y)$ can be derived from \cite{keshavan2010matrix}. Then we treat $p^{-1}P_{\bOmega}(\Y)$ as the perturbation for $\M_0$ as follows,
\begin{align*}
    p^{-1} P_{\bOmega}(\Y) = \M_0 + (p^{-1} P_{\bOmega}(Y) - \M_0).
\end{align*}
The Weyl-Wedin theorem assists in managing the Frobenius norm error for $\M^{(0)}$. We establish some new $L_{\infty}$ matrix perturbation bounds and apply them here to both control $\|\U^{(0)} - \U\|_{2,\infty}$ and $\|\V^{(0)} - \V\|_{2,\infty}$ , and subsequently $\|\M^{(0)} - \M_0\|_{\infty}$. 

The proof of Theorem \ref{thm:track_interation} is based on induction and consists of three main parts. First, we verify the efficiency of the pseudo-gradient utilized in our algorithm. Consider the perturbation formula,
\begin{align*}
    p^{-1} P_{\bOmega}(\M^{(k)} - \M_0 - \bH) = (\M^{(k)} - \M_0) + \left[p^{-1}P_{\bOmega}(\M^{(k)} - \M_0 - \bH) - (\M^{(k)} - \M_0)\right].
\end{align*}
By bounding the spectral norm of $p^{-1} P_{\bOmega}(\M^{(k)} - \M_0 - \bH) - (\M^{(k)} - \M_0)$ and applying the established $L_{\infty}$ matrix perturbation bounds, we can control the $L_2/L_{\infty}$ norm for the singular vectors of $P_{\bOmega}(\M^{(k)}-\M_0 -\bH)$ and their distances to the singular vectors of $\M^{(k)} - \M_0$. This allows us to achieve a sufficiently rapid reduction in the Frobenius norm error from $\|\M^{(k)} - \M_0\|_{F}$ to $\|\N^{(k+1)} - \M_0\|_{F}$. Second, we demonstrate that the low rank projection $\M^{(k+1)} = \operatorname{Proj}_{r}(\N^{(k+1)})$ has a minimal impact. 
This is because the leading singular space of the pseudo-gradient does not significantly deviate from the singular space of $\M^{(k)}$, resulting in only a minor truncation by the projection. Finally, we argue that the incoherent coefficients will not exhibit rapid increase from $\M^{(k)}$ to $\M^{(k+1)}$. Consider the perturbation formula given by 
\begin{align*}
    \N^{(k+1)} = \left(\N^{(k+1)} - \eta\mathcal{P}_{\U^{(k),\perp}}\widehat{\nabla} \mathcal{L}(\M^{(k)};\Y,\bOmega)\mathcal{P}_{\V^{(k),\perp'}}\right)&\\  +  \eta\mathcal{P}_{\U^{(k),\perp}} \widehat{\nabla} \mathcal{L}(\M^{(k)};\Y,\Omega)\mathcal{P}_{\V^{(k),\perp'}}&.
\end{align*}
The row and column norm of the perturbation term can be controlled. We subsequently employ the findings from \cite{fan2018eigenvector} to verify the incoherent condition. Then we can bound the maximum norm of $\M^{(k+1)} - \M_0$, and the induction for the Frobenius norm, $L_2/L_{\infty}$ norm, and maximum norm is completed.

\section{Algorithms for proposed estimators}
We provide the algorithm for the proposed estimator $\widetilde{\M}_{\text{nuc}}$ in \eqref{eq:our_estimator_convex}. The algorithm is designed for analyzing algorithm iterations and implementing in both simulated and real-world data. 
  \begin{breakablealgorithm}

  \caption{Iteration Algorithm for $\widetilde{\M}_{\text{nuc}}$}\label{alg:convex}
  \begin{algorithmic}[1]
  \REQUIRE Observed data $\Y\in \mathbb{R}^{m\times n}$, missing index matrix $\bOmega\in \mathbb{R}^{m\times n}$ and tuning parameter $\lambda$.
  \ENSURE Completion matrix $\M$.
  \STATE $\U^{(0)},\bm{D}^{(0)},\V^{(0)} \leftarrow \operatorname{svd}(p^{-1}\Y)$;
  \STATE $\M^{(0)} \leftarrow \U^{(0)}(\bm{D}^{(0)} - \lambda/2)_{+}\V^{(0)'}$;
  \STATE Sample $l$ standard Gaussian random matrix $\M_i\in \mathbb{R}^{m\times n}$ with singular value vector $\bm{\lambda}(\M_i),1\le i\le l$;
  \STATE $\widehat{\bm{\lambda}} \leftarrow \sum_{i=1}^l \bm{\lambda}(\M_i)/l$, $\operatorname{part\_sum} \leftarrow \sum_{i=n/3}^{2n/3} \widehat{\lambda}_i$;
  \WHILE {$k\le K$}
  \STATE $\U^{(k+1)},\bm{D}^{(k+1)},\V^{(k+1)}\leftarrow \operatorname{svd}(\Y - P_{\Omega}(\M^{(k)})$;
  \STATE $\widehat{\sigma}^{(k+1)} \leftarrow \sum_{i=n/3}^{2n/3}\bm{D}^{(k+1)}_{i,i}/\operatorname{part\_sum}$;
  \STATE $\widehat{\nabla}^{(k+1)}_{\M} \leftarrow \sum_{i=1}^n w_i(\bm{D}^{(k+1)}_{i,i} -  \widehat{\sigma}^{(k+1)}\widehat{\lambda}_i)\U^{(k+1)}_{[i]}\V^{(k+1)'}_{[i]}$;
  \STATE $\N^{(k+1)}\leftarrow \M^{(k)} - \eta_{k+1} P_{\bOmega}(\widehat{\nabla}_{\M}^{(k+1)})$;
  \STATE $\X^{(k+1)},\bm{\Lambda}^{(k+1)},\bm{Z}^{(k+1)}\leftarrow\operatorname{svd}(\N^{(k+1)})$;
  \STATE $\M^{(k+1)}\leftarrow \X^{(k+1)}(\bm{\Lambda}^{(k+1)} - \lambda/2)_{+}\bm{Z}^{(k+1)'}$;
  \ENDWHILE
  \RETURN $\M = \M^{(K+1)}$.
  \end{algorithmic}  
  \end{breakablealgorithm}
